# Supplementary material for: Bivariate change point detection in movement direction and speed
Source: arXiv:2402.02489 source file (2024-09-03)
Supplement: Supplementary file 1 [file Supplement2.tex]

\section*{Supplement 2: Details of the Recording and Post-processing}\label{appendix:datarecording}
	
	\subsection*{Data Acquisition}\label{appendix:acquisition}
	
	The data for organelle tracking was generated via light sheet-based fluorescence microscopy of 10-day old \textit{Arabidopsis thaliana} roots. The sample holder technique proposed by \cite{Wangenheim2015} was basis for sample preparation. Accordingly, the plants needed to be grown under sterile conditions on solid nutrient medium in a $45^{\circ}$-tilted manner within glass cuvettes with a diameter of 3 mm.
	
	The time laps data was recorded using a monolithic digital scanning light sheet-based fluorescence microscope \cite{Keller2010} combined with an EC Plan Neofluar 5x/0.16 air (Zeiss) lens for illumination and a WN Achroplan 40x/0.75 W (Zeiss) objective for detection of the fluorescence. Excitation wave length of 488 nm and detection between 500 and 550 nm utilizing a bandpass filter 525/47 were applied to image GFP-fluorescence, while 561 nm excitation wave length and 607/70 bandpass filter were used to image mCherry-fluorescence. The exposure time of the laser was kept to 20 ms. The data was collected utilizing an EMCCD camera compiling a display window for the used objective of 224.46 $\mu$m x 168.7 $\mu$m, which is composed of 1392 x 1040 pixels, therefore the resolution is 0.16125 $\mu m$.
	
	To image living organelles in roots, fluorescent marker lines generated by tDNA insertion were used. To visualise plastids, the fluorescent marker protein GFP was fused to the plastid transport signal sequence (tp), which is used in nature to target the small subunit (SSU) of the protein Rubisco to the plastid (tpSSU-GFP). To fluorescently stain peroxisomes, the peroxisome targeting signal SKL was fused to the fluorescent marker mCherry (mCherry-SKL). Both plant lines were selected by BASTA resistance.
	
	Image data was acquired of both marker lines by imaging 30 $\mu$m deep into the mature zone of the root in 1 $\mu$m steps, resulting in a stack of 31 two-dimensional greyscale microscopy images. A stack was recorded each 4.3 seconds, for the plastid marker line over a time course of 1 h resulting in 841 timepoints, while the peroxisome marker line was recorded for 30 min generating a set of 421 time points.

	\subsection*{Detection and Tracking}
	
	\label{appendix:detectiontracking}
	
	Detection and tracking was done as follows. Peroxisome movement was tracked using the software Arivis Vision 4D Version 3.5.1. After converting the data into .sis format via the arivis SIS Converter, the data was first segmented to create digital objects for each peroxisome by using the implemented ''blob finder'' function. As settings for the blob finder for the peroxisome data a diameter  1.2 $\mu$m for tracking, a probability threshold of 20 \% and a split sensitivity of 70 \% for tracking were applied. The segmented objects were interconnected over each time point by hand, making use of the 3D viewer function of the software, gaining a table of the 3-dimensional coordinates of each peroxisome over time.\\
	
	Detection and tracking of the plastides was performed using the TrackMate Plugin (version=4.0.1) \citep{trackmate} of FIJI \cite{FIJI}. For the particle detection step the Laplacian of Gaussian Detector (LoG Detector) was used, which applies a Gaussian filter to the image and then uses the parameter "radius" to identify local maxima (light spots in front of darker background) as spots, we chose radius$=2\mu m$. Each spot has a quality value, which is a measure of how sure the algorithm is to have identified a ''True'' spot. Since we have a stack of microscopy images for each time point our spots are technically balls. After selecting a lower threshold for the quality parameter by visually checking the effect of different thresholds, the detection is executed on the image stack for each time point resulting in spacio-temporal coordinates (t,x,y,z) per detected spot.
	
	For the tracking the LAP Tracker (Linear Assignment Tracker) was used. This Tracker considers the spots from two consecutive time points $t$ and $t+1$. For each possible Spot pair $(s_t,s_{t+1})$ the Tracker assigns a cost value for linking based on the euclidean distance between the spots. Then the linking configuration with the minimum cost between the spots from time $t$ to $t+1$ is chosen. This is repeated for every consecutive time point pair, resulting in time series of spots. For a more detailed explanation of the algorithms as well as the usage of the software see the TrackMate entry of the FIJI website \cite{FIJI} and the documentation which can be found on the website.
	
	The settings used for detection and tracking in the TrackMate Plugin for Fiji (version 4.0.1) were as follows. For the LoG detector, median filtering was off, sub-pixel localisation was allowed, and we used values of radius of 2 $\mu m$, target channel of $1$ and a threshold of zero. For the spot filter collection, the quality was set to $\ge 18.2$ and the estimated diameter to $\ge 2.0 \mu m$. For the LAP tracker, track splitting and merging was not allowed, the maximal linking distance and gap closing distance were $15 \mu m$ and the maximum frame gap was $2$.		
	
	\subsection*{Post-Processing}
	
	\label{appendix:postprocessing}
	
	Since we obtained the plastid movement tracks by using automated tracking with the LAP-tracking algorithm from the TrackMate Plugin, which in general "rarely gives an error free result" \cite{Beltman2009}, we post-processed the tracks.
	
	First we made two quick adjustments to the data set. Since we are interested in the long-term behaviour of plastide movements, we chose to keep only tracks with recording times longer than 100 time points. Then we discarded tracks which contained so-called {border tracking}. {Border tracking} \cite{Beltman2009} occurs when cell organelles move outside the rectangular cuboid of the microscopy area. The position of a cell organelle is detected by finding its centre of mass, but since the fluorescence of the cell organelles slightly outside the microscopy area still spreads into it, their position will wrongly be detected as moving exactly in the border plane of the microscopy area. This leads to skewed results when characterizing the movement. Therefore, these tracks were discarded.
	
	The resulting tracks were individually analysed and corrected by hand due to smaller artefacts.  For every track $T$ we selected the set $S_T$ of all tracks observed within a certain small neighborhood of this track. We then investigated the 3D plot of these tracks as well as the process of their signal-to-noise ratios and step lengths between subsequent positions. We then performed three steps to eliminate three different artifacts. 
 
 First, the tracking algorithm globally minimizes the links between positions at time $t$ and $t+1$. If an organelle is  detected at time $t$ but not at time $t+1$, the algorithm may falsely assign another organelle to the same track, which may lead to isolated long jumps. If short peaks in the step length occurred when the plastide associated with the reference track was not detected, we separated the track and used the remaining parts individually if they were longer than 100 time points. 
 
Second, {track switching} (\cite{Beltman2009}) can occur when two plastides come into close proximity. The tracking algorithm, favouring short links, may then link the further movement of track $a$ with the start from track $b$, i.e. switching the first and second part of the two tracks. In our data, temporary close proximity of tracks was sometimes followed by a sudden switch in the level of the signal-to-noise ratios as well as a change in the step lengths. In these cases, we switched the tracks at the respective time. 
Third, double tracking (\cite{Beltman2009}) can occur when during spot detection the plastide, which can deform from vaguely spherical to stretched shape, was accidentally detected as two plastides. In our data set, some tracks suddenly stopped, where at the same time one of the near tracks started in very close proximity. If this occurred and if the signal-to-noise ratio and the step length of both tracks behaved  similarly, we connected the two tracks. This post-processing led to the final plastid data set of tracks used for analysis.
